# Supplementary material for: Application Performance Modeling via Tensor Completion
Source: arXiv:2210.10184 source file (2023-08-29)
Supplement: Supplementary file 1 [file appendix.tex]

\subsection{Error Metrics}
We consider aggregate error metrics that address the asymmetry and biased under-prediction of MAPE discussed in Section \ref{sec:review:assessment} and summarized in Table \ref{error_metric_table}.
We demonstrate the equivalence of SMAPE, MLogQ, and LGMAPE to first-order approximation for small relative errors.
Given a collection of measured configurations $\{(\mathbf{x}_{k},y_{k})\}_{k=1}^{M}$ and corresponding model predictions $\{(\mathbf{x}_{k},m_{k}))\}_{k=1}^{M}$, 
we consider the following:
\begin{align}
    \mathbf{MAPE}&\coloneqq \frac{1}{M}\cdot\sum_{k=1}^{M} |m_{k}-y_{k}|/y_{k}\\
    \mathbf{SMAPE}&\coloneqq\frac{2}{M}\cdot\sum_{k=1}^{M} |m_{k}-y_{k}|/(y_{k}+m_{k})\\
    \mathbf{MLogQ}&\coloneqq\frac{1}{M}\cdot\sum_{k=1}^{M} |\log(m_{k}/y_{k})|\\
    \mathbf{MLogQ2}&\coloneqq\frac{1}{M}\cdot\sum_{k=1}^{M} \log^{2}(m_{k}/y_{k})\\
    \mathbf{LGMAPE}&\coloneqq\frac{1}{M}\cdot\sum_{k=1}^{M} \log(|m_{k}-y_{k}|/y_{k})
\end{align}
Any execution-time prediction $m\equiv y(1+\epsilon)$ is equivalent to a latent \textit{true} execution-time $y$ multiplied by some error $(1+\epsilon)$, where $\epsilon$ is the relative error.

\begin{align*}
\textbf{MAPE}&\coloneqq\frac{1}{M}\sum_{k=1}^{M}\frac{|m_{k}-y_{k}|}{y_{k}}\\
&=\frac{1}{M}\sum_{k=1}^{M}\frac{|y_{k}(1+\epsilon_{k})-y_{k}|}{y_{k}}\\
&=\frac{1}{M}\sum_{k=1}^{M}|1+\epsilon_{k}-1|\\
&=\frac{1}{M}\sum_{k=1}^{M}|\epsilon_{k}|\\
\end{align*}
We remark that minimization of SMAPE implies minimization of LGMAPE, as minimization of SMAPE relies solely on minimization of $\epsilon_{k}$, which leads to $2+\epsilon\approx 2$.

\begin{align*}
\textbf{LGMAPE}&\coloneqq\log\left(\left(\prod_{k=1}^{M}\left(\frac{|m_{k}-y_{k}|}{y_{k}}\right)\right)^{\frac{1}{M}}\right)\\
&=\frac{1}{M}\sum_{k=1}^{M}\log(\frac{|m_{k}-y_{k}|}{y_{k}})\\
&=\frac{1}{M}\sum_{k=1}^{M}\log\left(\left|\frac{m_{k}}{y_{k}}-1\right|\right)\\
&=\frac{1}{M}\sum_{k=1}^{M}\log\left(\left|\frac{y_{k}(1+\epsilon_{k})}{y_{k}}-1\right|\right)\\
&=\frac{1}{M}\sum_{k=1}^{M}\log(|1+\epsilon_{k}-1|)\\
&=\frac{1}{M}\sum_{k=1}^{M}\log(|\epsilon_{k}|)\\
\end{align*}
We remark that a model that minimizes LGMAPE is equivalent to one that minimizes $\frac{1}{M}\sum_{k=1}^{N}|\epsilon_{k}|$, as log applies a monotonic transformation.
% Each term will be negative.
% No obvious minimum.

\begin{align*}
\textbf{SMAPE}&\coloneqq\frac{2}{M}\sum_{k=1}^{M}\frac{|m_{k}-y_{k}|}{m_{k}+y_{k}}\\
&=\frac{2}{M}\sum_{k=1}^{M}\frac{|y_{k}(1+\epsilon_{k})-y_{k}|}{y_{k}(1+\epsilon_{k})+y_{k}}\\
&=\frac{2}{M}\sum_{k=1}^{M}\frac{|1+\epsilon_{k})-1|}{1+\epsilon_{k}+1}\\
&=\frac{2}{M}\sum_{k=1}^{M}\frac{|\epsilon_{k}|}{2+\epsilon_{k}}\\
\end{align*}
We remark that minimization of SMAPE implies minimization of LGMAPE, as minimization of SMAPE relies solely on minimization of $\epsilon_{k}$, which leads to $2+\epsilon\approx 2$.

\begin{align*}
\textbf{MLogQ}&\coloneqq\frac{1}{M}\sum_{k=1}^{M}\left|\log\left(\frac{m_{k}}{y_{k}}\right)\right|\\
&=\frac{1}{M}\sum_{k=1}^{M}\left|\log\left(\frac{y_{k}(1+\epsilon_{k})}{y_{k}}\right)\right|\\
&=\frac{1}{M}\sum_{k=1}^{M}|\log(1+\epsilon_{k})|\\
&\approx\frac{1}{M}\sum_{k=1}^{M}\left|\frac{\epsilon_{k}}{1+\epsilon_{k}}\right|\\
\end{align*}
We remark that minimization of MLogQ implies minimization of LGMAPE, as minimization of MLogQ relies solely on minimization of $\epsilon_{k}$, which leads to $1+\epsilon\approx 1$.

\begin{align*}
\textbf{MLogQ2}&\coloneqq\frac{1}{M}\sum_{k=1}^{M}\log\left(\frac{m_{k}}{y_{k}}\right)^{2}\\
&=\frac{1}{M}\sum_{k=1}^{M}\log\left(\frac{y_{k}(1+\epsilon_{k})}{y_{k}}\right)^{2}\\
&=\frac{1}{M}\sum_{k=1}^{M}\log(1+\epsilon_{k})^{2}\\
&\approx\frac{1}{M}\sum_{k=1}^{M}\left(\frac{\epsilon_{k}}{1+\epsilon_{k}}\right)^{2}\\
\end{align*}
We remark that minimization of MLogQ2 is not equivalent to minimization of the other error metrics.
MLogQ2 is instead approximately equal to the square of the Frobenius norm of the relative errors $\epsilon_{k}$. % and is equivalent to the application of least-squares to the log of the multiplicative factors.

\subsection{Loss Function Derivations}
\begin{comment}
    The scalar expressions for $\nabla f_{\phi}(\mathbf{U})=0$ expose dependencies among the unknowns:
    \begin{align}
        \frac{\partial f_{\phi}(u_{i,r})}{\delta u_{i,r}} &= \sum_{(j,k)\in\Omega_{i}} 2\phi(t_{i,j,k},\sum_{a=1}^{R}u_{i,a}v_{j,a}w_{k,a})\frac{\partial \phi}{\partial u_{i,r}} + 2\lambda u_{i,r}=0\\
    \end{align}
\end{comment}
  Using notation introduced in Section \ref{sec:tc}, we formulate low-rank tensor models for accurate execution time prediction by minimizing the following objective functions:
  $f_{\phi_{1}}(U,V,W)=$
    \begin{align}
        \lambda(||\mathbf{U}||_{F}^{2}+||\mathbf{V}||_{F}^{2}+||\mathbf{W}||_{F}^{2})+\sum_{(i_{1},i_{2},i_{3})\in \Omega} \left(\log(t_{i_{1},i_{2},i_{3}}) - m_{i_{1},i_{2},i_{3}}\right)^{2}%.\langle \mathbf{u}_{i_{1}},\mathbf{v}_{i_{2}},\mathbf{w}_{i_{3}}\rangle).
    \end{align}
    and $f_{\phi_{2}}(U,V,W)=$
    \begin{align}
        \lambda(||\mathbf{U}||_{F}^{2}+||\mathbf{V}||_{F}^{2}+||\mathbf{W}||_{F}^{2})+\sum_{(i_{1},i_{2},i_{3})\in \Omega} \left(\log(t_{i_{1},i_{2},i_{3}}) - \log(m_{i_{1},i_{2},i_{3}})\right)^{2}\\
        -\eta\left(\sum_{i_{1}=1}^{I_{1}}\sum_{r=1}^{R} \log(u_{i_{1},r}) + \sum_{i_{2}=1}^{I_{2}}\sum_{r=1}^{R} \log(v_{i_{2},r}) + \sum_{i_{3}=1}^{I_{3}}\sum_{r=1}^{R} \log(w_{i_{3},r})\right).\nonumber%.\langle \mathbf{u}_{i_{1}},\mathbf{v}_{i_{2}},\mathbf{w}_{i_{3}}\rangle).
    \end{align}
    Objective function $f_{\phi_{2}}$ directly minimizes error metric MLogQ2, while both $f_{\phi_{1}}$ and $f_{\phi_{2}}$ indirectly minimize error metric MLogQ, which we report in all experimental results.

  The following expressions are used to minimize $f_{\phi_{1}}(\mathbf{U},\mathbf{V},\mathbf{W})$ via the Alternating Least-Squares (ALS) method: $\nabla f_{\phi_{1}}(\mathbf{u}_{i_{1}}) =$
  \begin{align}
    \sum_{(i_{2},i_{3})\in\Omega_{i}} 2(\log(t_{i_{1},i_{2},i_{3}})-m_{i_{1},i_{2},i_{3}})(\mathbf{v_{i_{2}}}\odot\mathbf{w_{i_{3}}}) + 2\lambda \mathbf{u_{i_{1}}}
  \end{align}
  and $H_{f_{\phi_{1}}}(\mathbf{u}_{i_{1}})=$
  \begin{align}
    \sum_{(i_{2},i_{3})\in \Omega_{i_{1}}} -2(\mathbf{v_{i_{2}}}\odot\mathbf{w_{i_{3}}})(\mathbf{v_{i_{2}}}\odot\mathbf{w_{i_{3}}})^{T} + 2\lambda \mathbf{I}
  \end{align}
  As the objectives $f_{\phi_{2}}(\mathbf{u}_{i_{1}}),f_{\phi_{2}}(\mathbf{v}_{i_{2}}),f_{\phi_{2}}(\mathbf{w}_{i_{3}})$ are quadratic, a single Newton iteration suffices.

  The following expressions are used to minimize $f_{\phi_{2}}(\mathbf{U},\mathbf{V},\mathbf{W})$ via alternating minimization via Newtons Method (AMN): $\nabla f_{\phi_{2}}(\mathbf{u}_{i_{1}})=$
  \begin{align}
    \sum_{(i_{2},i_{3})\in\Omega_{i_{1}}} 2(\log(t_{i_{1},i_{2},i_{3}})-\log(m_{i_{1},i_{2},i_{3}}))\frac{-(\mathbf{v}_{i_{2}}\odot\mathbf{w}_{i_{3}})}{m_{i_{1},i_{2},i_{3}}}\\
    +2\lambda \mathbf{u}_{i_{1}} -\eta\frac{1}{\mathbf{u}_{i_{1}}}.\nonumber
  \end{align}
  and $H_{f_{\phi_{2}}}(\mathbf{u_{i_{1}}})=$
  \begin{align}
    \sum_{(i_{2},i_{3})\in \Omega_{i_{1}}} 2\frac{1+\log(t_{i_{1},i_{2},i_{3}})-\log(m_{i_{1},i_{2},i_{3}})}{m_{i_{1},i_{2},i_{3}}^{2}}(\mathbf{v}_{i_{2}}\odot\mathbf{w}_{i_{3}})(\mathbf{v}_{i_{2}}\odot\mathbf{w}_{i_{3}})^{T}\\
    + 2\lambda \mathbf{I} +\eta \mathbf{I}\odot\left(\frac{1}{\mathbf{u}_{i_{1}}}\left(\frac{1}{\mathbf{u}_{i_{1}}}\right)^{T}\right).\nonumber
  \end{align}
  As the objectives $f_{\phi_{1}}(\mathbf{u}_{i_{1}}),f_{\phi_{1}}(\mathbf{v}_{i_{2}}),f_{\phi_{1}}(\mathbf{w}_{i_{3}})$ are nonlinear (but generally convex), many iterations of Newton iterations are necessary.
  Thus, for CP rank 1, $\frac{\partial f_{\phi_{2}}}{\partial u_{i_{1}}}(u_{i_{1}})=$
  \begin{align*}
  \sum_{(i_{2},i_{3})\in\Omega_{i_{1}}} 2(\log(t_{i_{1},i_{2},i_{3}})-\log(m_{i_{1},i_{2},i_{3}}))\frac{-v_{i_{2}}w_{i_{3}}}{m_{i_{1},i_{2},i_{3}}}+2\lambda u_{i_{1}} -\eta\frac{1}{u_{i_{1}}}
  \end{align*}
  and $H_{f_{\phi_{2}}}(u_{i_{1}})=$
  \begin{align*}
  \sum_{(i_{2},i_{3})\in \Omega_{i_{1}}} 2\frac{1+\log(t_{i_{1},i_{2},i_{3}})-\log(m_{i_{1},i_{2},i_{3}})}{m_{i_{1},i_{2},i_{3}}^{2}}(v^{2}_{i_{2}} w^{2}_{i_{3}})+ 2\lambda +\frac{\eta}{u^{2}_{i_{1}}}.
  \end{align*}

    {\color{red}
    Any connection between loss function and requisite density?
    No, seems like loss 2 is more accurate relative to rank, but both reach the same test error given the same training samples.
    Obviously, we'd like to use a larger tensor to mitigate quadrature/interpolation error, but if the tensor is too sparse, we incur too much completion error.
    Start with a comparison of the error for T=256 samples for a 32x32x32 tensor for both loss functions. Which incurs smaller error?
    }

\subsection{Comparison to Analytic Cost Models}

    \begin{figure}[t] 
        \centering
        \includegraphics[width=1\linewidth]{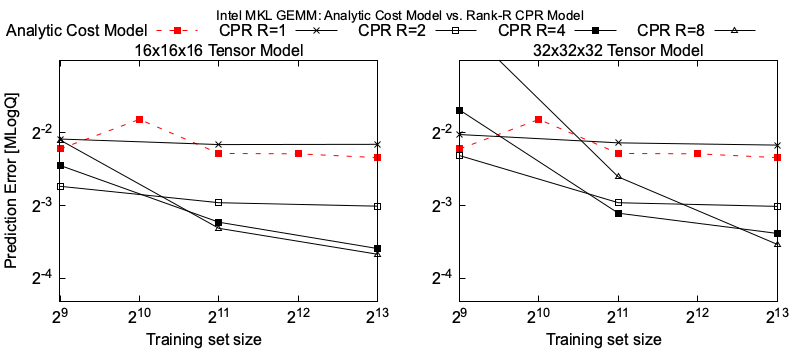} 
        \caption{...}
        %\label{plot:error_vs_refinement_opt_time} 
    \end{figure}

An analytic cost model for matrix multiplication $C_{m\times n}\gets A_{m\times k}B_{k\times n}$ under the assumption of a 2-level memory hierarchy with cache size $H$ might be:
\begin{align*}
T_{\text{GEMM}}=\delta mnk + \beta (mn+nk+mk+\frac{mnk}{\sqrt{H}})
\end{align*}

We can refactor this cost expression into a rank-1 model as follows:
\begin{align*}
\hat{T}_{\text{GEMM}}\approx(\alpha_{1}m+\alpha_{2})(\alpha_{1}n+\alpha_{2})(\alpha_{1}k+\alpha_{2})
\end{align*},
where $\alpha_{1}=(\delta + \beta H^{-1/2})^{1/3}$ and $\alpha_{2}=\beta (\delta + \beta H^{-1/2})^{-2/3}$.
Taking a log-transformation of data assumed to be generated by the initial cost model would increase the requisite rank (up to rank 5) necessary to capture a significant portion of the variation in execution times using a low-rank tensor model, and therefore exemplifies the benefits of minimizing the $f_{\phi_{2}}$ objective function as opposed to the $f_{\phi_{1}}$ objective function.

This example highlights the ability of CPR to automatically derive (global) analytic cost models with CP rank 1 given a sufficient number of training samples.
Test accuracy may be further improved by increasing CP rank and thereby uncovering more accurate cost models.
